# Supplementary material for: Experimental quasi-1D capillary-wave turbulence
Source: arXiv:2110.01448 source file (2021-10-01)
Supplement: Supplementary file 1 [file Supplemental2.pdf]

# Supplemental Material
# "Experimental quasi-1D capillary-wave turbulence"

Guillaume Ricard and Eric Falcon
*Université de Paris, MSC, UMR 7057 CNRS, F-75 013 Paris, France*

In this Supplemental Material, we present additional data analyses related to the observation of quasi-1D capillary-wave turbulence: a movie (Sec. I), the wave elevation distribution probability (Sec. II), the power spectrum of the wave elevation for a monochromatic forcing (Sec. III), low- and high-order correlations of the wave elevation (Sec. IV-V), and decaying experiments to infer the nonlinear and dissipative timescales (Sec. VI). Notations as in the aforementioned manuscript.

## I. MOVIE

*Filename:* WT1DMercuryView1.mp4
*Duration:* 21s
*Filesize:* 5.6 Mo
*Description:* Running experiment for 1D capillary-wave turbulence. Mainly gravity-capillary waves are visible by eyes. Random forcing frequency of the paddle: $2 \leq f \leq 5$ Hz. Wave steepness $\epsilon = 0.06$. The wave elevation, $\eta(t)$, is measured with a wire gauge (located at the center of the tank). The spatio-temporal measurement, $\eta(x,t)$, with the lateral camera is not visible. The sealed cover used for security purposes has been removed to take videos.

## II. WAVE ELEVATION PROBABILITY DISTRIBUTION

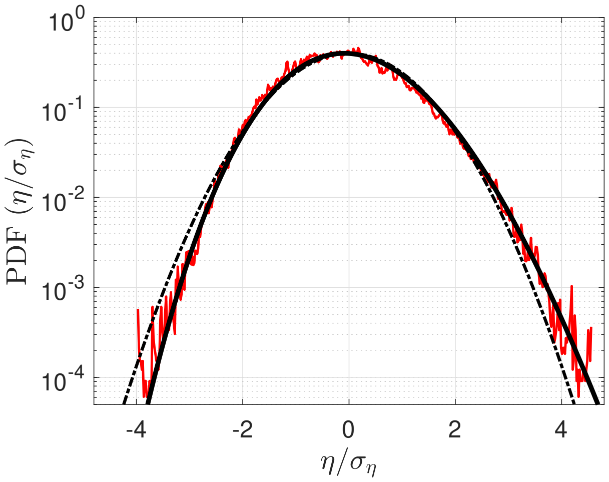


Figure S1: Probability distribution function (PDF) of normalized wave elevation $\eta(t)/\sigma_\eta$ recorded during 15 min. $\sigma_\eta = 0.85$ mm. Wave steepness $\epsilon = 0.06$. Dash-dotted line displays a Gaussian distribution of zero mean and unit standard deviation. Solid line shows a Tayfun distribution for $\epsilon = 0.06$. A weak flatness (kurtosis $K = \langle\eta^4\rangle/\langle\eta^2\rangle^2 = 3.08$) and a weak asymmetry (skewness $Sn = \langle\eta^3\rangle/\langle\eta^2\rangle^{3/2} = 0.26$) is observed as expected for a weakly nonlinear gravity-capillary wave field.

## III. POWER SPECTRUM OF WAVE ELEVATIONS FOR A MONOCHROMATIC FORCING

.

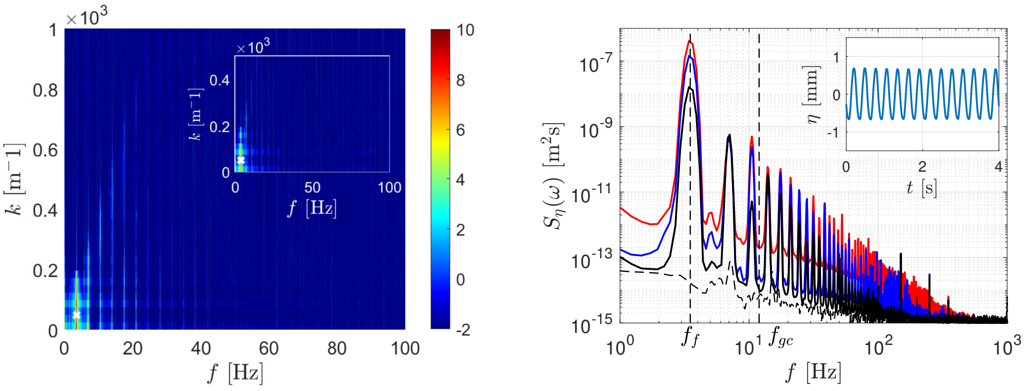


Figure S2: Sinusoidal forcing at $f_f = 3.5$ Hz (white rectangle). **Left**: Spatio-temporal power spectrum $S_\eta(k,\omega)$ of wave elevation. No wave turbulence regime is observed, only a set of discrete peaks corresponding to the forcing harmonics. Wave steepness $\epsilon = 0.06$. Inset: same for $\epsilon = 0.03$. Log colorbar. **Right**: Temporal power spectra $S_\eta(k,\omega)$ computed from the single-point measurement (capacitive gauge) for different $\epsilon = 0.006$, 0.03, and 0.06 (from bottom to top curves). Only harmonics of the forcing appear in the spectra, and no continuous cascade is observed. Bottom curve corresponds to the experimental noise (no forcing). Inset: typical temporal evolution of the wave elevation obtained from the capacitive gauge for $\epsilon = 0.06$.

## IV. LOW-ORDER CORRELATIONS OF THE WAVE ELEVATION

In this section, we briefly present additional results of low-order correlations ($N = 3$ and $N = 4$).

### A. Bicoherence

Three-wave *resonant* interactions and three-wave *quasi-resonant* interactions read, respectively

$$\omega_1(k_1) + \omega_2(k_2) - \omega_3(k_1 + k_2) = 0 \ , \tag{s1}$$

$$\omega_1(k_1) + \omega_2(k_2) - \omega_3(k_1 + k_2) < \delta_\omega \ . \tag{s2}$$

They are quantify by bicoherence, computed using Eq. (4), and are shown in Fig. S3.

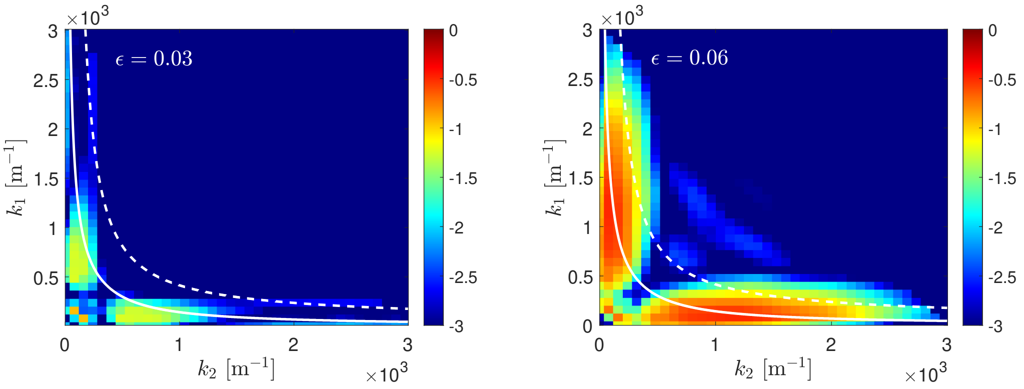


Figure S3: Bicoherence $B(k_1, k_2)$ for different values of $\epsilon$. Solid lines: three-wave *resonant* interactions, solutions of Eq. (s1) with $\omega_i^2 = gk_i + (\gamma/\rho)k_i^3$. Dashed lines: border of the three-wave *quasi-resonant* interaction area, solutions of Eq. (s2) with $\omega_i^2 = gk_i + (\gamma/\rho)k_i^3$. Nonlinearity increases the number of quasi-resonances. Log colorbar.

## B. Tricoherence

Four-wave *resonant* interactions and four-wave *quasi-resonant* interactions for a $2 \leftrightarrow 2$ process (i.e. $k_1+k_2 = k_3+k_4$) read, respectively

$$\omega_1(k_1) + \omega_2(k_2) - \omega_3(k_3) - \omega_4(k_1 + k_2 - k_3) = 0 \; , \tag{s3}$$
$$\omega_1(k_1) + \omega_2(k_2) - \omega_3(k_3) - \omega_4(k_1 + k_2 - k_3) < \delta_\omega \; . \tag{s4}$$

They are quantify by tricoherence, computed using Eq. (5), and are shown in Fig. S4.

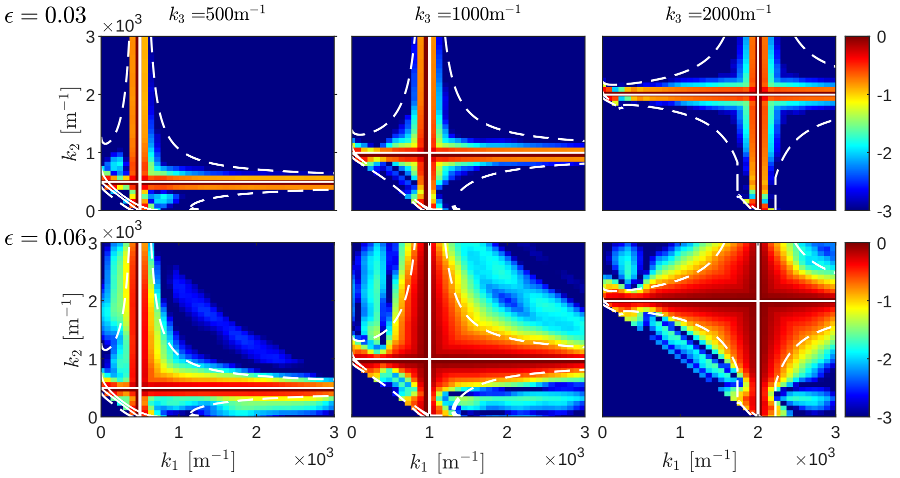


Figure S4: Tricoherence $T_{2\leftrightarrow 2}(k_1, k_2, k_3)$ for different values of $k_3$ and $\epsilon$. $2 \leftrightarrow 2$ process. Solid lines: four-wave *resonant* interactions, solution of Eq. (s3) with $\omega_i^2 = gk_i + (\gamma/\rho)k_i^3$. Dashed lines: borders of four-wave *quasi-resonant* interaction area, solutions of Eq. (s4) with $\omega_i^2 = gk_i + (\gamma/\rho)k_i^3$. Nonlinearity clearly increases the number of quasi-resonances. Log colorbar.

We discuss now the possible occurrence of four-wave interactions involving a $3 \leftrightarrow 1$ process (i.e. $k_1 + k_2 + k_3 = k_4$). The corresponding four-wave *resonant* interactions and 4-wave *quasi-resonant* interactions then read, respectively

$$\omega_1(k_1) + \omega_2(k_2) + \omega_3(k_3) - \omega_4(k_1 + k_2 + k_3) = 0 \; , \tag{s5}$$
$$\omega_1(k_1) + \omega_2(k_2) + \omega_3(k_3) - \omega_4(k_1 + k_2 + k_3) < \delta_\omega \; . \tag{s6}$$

The corresponding tricoherence is computed as

$$T_{3\leftrightarrow 1}(k_1, k_2, k_3) = \frac{|\langle \eta_{k_1}\eta_{k_2}\eta_{k_3}\eta^*_{k_1+k_2+k_3}\rangle|}{\sqrt{\langle |\eta_{k_1}\eta_{k_2}|^2\rangle \langle |\eta_{k_3}\eta_{k_1+k_2+k_3}|^2\rangle}} \; , \tag{s7}$$

and are shown in Fig. S5.

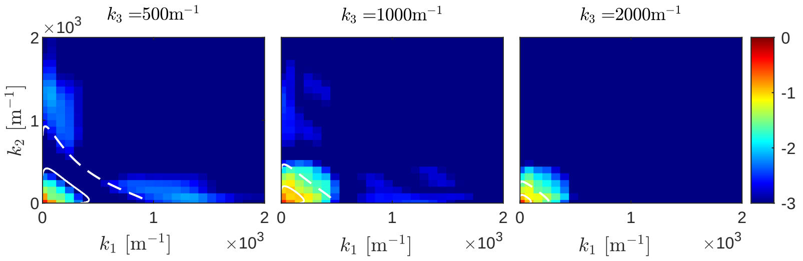


Figure S5: Tricoherence $T_{3\leftrightarrow 1}(k_1, k_2, k_3)$ for different value of $k_3$ at fixed $\epsilon = 0.06$. $3 \leftrightarrow 1$ process. The values obtained are much smaller than for the $2 \leftrightarrow 2$ process of Fig. S4. Solid line: four-wave *resonant* interactions, solutions of Eq. (s5) with $\omega_i^2 = gk_i + (\gamma/\rho)k_i^3$. Dashed lines: borders of four-wave *quasi-resonant* interaction area, solutions of Eq. (s6) with $\omega_i^2 = gk_i + (\gamma/\rho)k_i^3$. Almost no $3 \leftrightarrow 1$ process occurs in the capillary regime ($k > k_{gc} \simeq 575$ m$^{-1}$). Log colorbar.

## V. HIGH-ORDER CORRELATIONS OF THE WAVE ELEVATION

We present additional results on quadricoherence that highlights five-wave interactions. Five-wave *resonant* interactions and five-wave *quasi-resonant* interactions, for a $3 \leftrightarrow 2$ process (i.e. $k_1 + k_2 + k_3 = k_4 + k_5$), read respectively

$$\omega_1(k_1) + \omega_2(k_2) + \omega_3(k_3) - \omega_4(k_4) - \omega_5(k_1 + k_2 + k_3 - k_4) = 0 \ , \quad \text{(s8)}$$

$$\omega_1(k_1) + \omega_2(k_2) + \omega_3(k_3) - \omega_4(k_4) - \omega_5(k_1 + k_2 + k_3 - k_4) < \delta_\omega \ . \quad \text{(s9)}$$

Quadricoherence is computed for fixed $k_3$ and $k_4$. For $k_4 \ll k_3$, Fig. S6a shows results close to the ones of Fig. S5 for a $N = 4$ ($3 \leftrightarrow 1$) process. For $k_4 \gg k_3$, Fig. S6b shows results close to the ones of Fig. S4 for a $N = 4$ ($2 \leftrightarrow 2$) process.

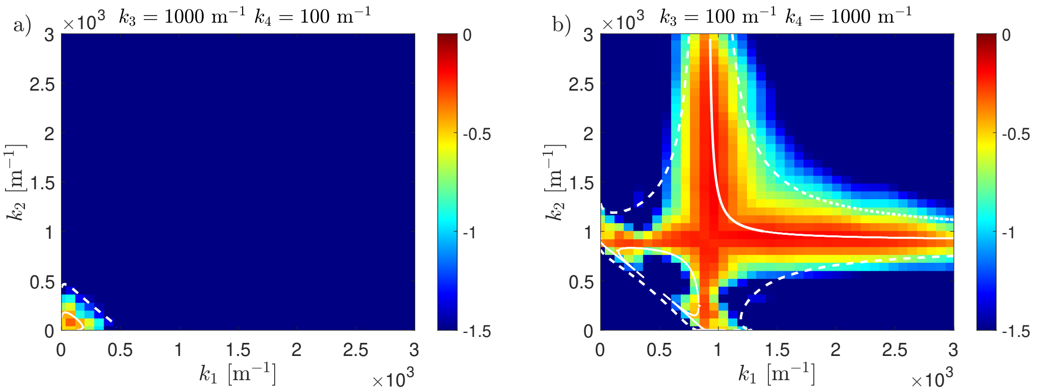


Figure S6: Quadricoherence $Q_{3\leftrightarrow 2}(k_1, k_2, k_3, k_4)$ for different values of $k_3$ and $k_4$ at fixed $\epsilon = 0.06$. $3 \leftrightarrow 2$ process. Solid line: five-wave resonant interactions, solutions of Eq. (s8) with $\omega_i^2 = gk_i + (\gamma/\rho)k_i^3$. Dashed lines: borders of the five-wave quasi-resonant interaction area, solutions of Eq. (s9) with $\delta_\omega = 40$ Hz and $\omega_i^2 = gk_i + (\gamma/\rho)k_i^3$. Log colorbar.

Finally, quadricoherence computed for a $4 \leftrightarrow 1$ process for $N = 5$ leads to a similar conclusion than for the $3 \leftrightarrow 1$ process for $N = 4$, and is even more negligible (not shown).

## VI. DECAYING EXPERIMENTS

.

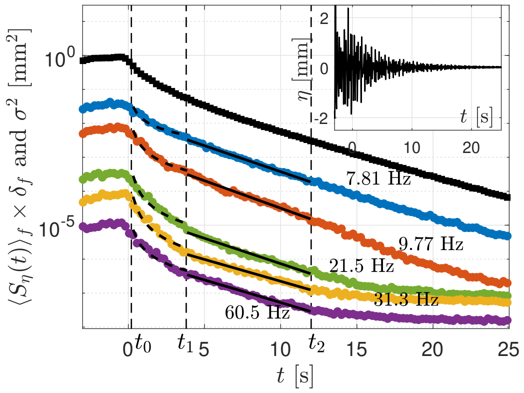


Figure S7: Wave turbulence decaying experiments. Decay of the total wave energy $\sigma_\eta^2(t)$ (top curve) and of the Fourier modes $S_\eta(f^\star, t)\delta_f$ for increasing frequencies $f^\star$ (from top to bottom curves). $\delta f \equiv 1/\delta t$ with $\delta t = 0.25$ s the temporal step. The results are averaged over 250 decay experiments. Dashed vertical lines delimit the fast power-law decay [dashed-line fits between $t_0$ and $t_1$ to infer $\tau_{nl}(f^\star)$], and the slow exponential decay [solid-line fits between $t_1$ and $t_2$ to infer $\tau_{diss}(f^\star)$]. Timescales $\tau_{nl}(f^\star)$ and $\tau_{diss}(f^\star)$ are found to be roughly independent of the $f^\star$ scale (see article). Inset: Typical temporal decay of wave elevation signal measured with the wire gauge. Random forcing is stopped at $t = 0$ s.
